# Supplementary material for: Anomalous diffusion and ergodicity breaking in heterogeneous diffusion processes
Source: arXiv:1303.5533 source file (2013-03-22)
Supplement: Supplementary file 1 [file supp.pdf]

# Supplementary Material
# Anomalous diffusion and ergodicity breaking in heterogeneous diffusion processes

Andrey G. Cherstvy,[1] A. V. Chechkin,[2,3] and R. Metzler[1,4]

[1]*Institute for Physics & Astronomy, University of Potsdam, 14476 Potsdam-Golm, Germany*
[2]*Akhiezer Institute for Theoretical Physics, Kharkov Institute of Physics and Technology, Kharkov 61108, Ukraine*
[3]*Max-Planck Institute for the Physics of Complex Systems, Nöthnitzer Straße 38, 01187 Dresden, Germany*
[4]*Department of Physics, Tampere University of Technology, 33101 Tampere, Finland*

(Dated: 21st March 2013)

We provide details of the derivation of various results quoted in the main text and introduce an approximative scheme to calculate the moments of the HDP process. Moreover, we discuss the velocity autocorrelation function.

*Probability density function (PDF).* To solve the Langevin equation $\dot{x}(t) = \sqrt{2D(x)}\zeta(t)$ in the Stratonovich sense we introduce the new variable [1]

$$y(x) = \int^x \frac{dx'}{\sqrt{2D(x')}} = \frac{\sqrt{2/A}}{2-\alpha}|x|^{(2-\alpha)/2}\mathrm{sign}(x), \quad \text{(S1)}$$

where $y(t)$ is the Wiener process with the known Gaussian PDF for the initial condition $y(0) = 0$, namely,

$$P(y,t) = \frac{1}{\sqrt{2\pi t}}\exp\left(-\frac{y^2}{2t}\right). \quad \text{(S2)}$$

Returning to the $x$-variable yields the PDF (2)

With the back-transformation $y \to x$, from Eq. (S1) we find that $x(t) = 2^{p/2}p^{-p}|y|^p\mathrm{sign}(y)$, and the autocorrelation function is evaluated via the 2-point probability density function for the Wiener process,

$$\langle x(t_1)x(t_2)\rangle = \frac{2^p}{p^{2p}}\int_{-\infty}^{\infty}dy_1\int_{-\infty}^{\infty}dy_2 P(y_1,t_1) \times\mathrm{sign}(y_1)\mathrm{sign}(y_2)|y_1|^p|y_2|^p\pi(y_2,t_2|y_1,t_1), \quad \text{(S3)}$$

where we used the transition probability

$$\pi(y_2,t_2|y_1,t_1) = \frac{1}{\sqrt{2\pi(t_2-t_1)}}\exp\left(-\frac{(y_2-y_1)^2}{2(t_2-t_1)}\right). \quad \text{(S4)}$$

Evaluating the integral in Eq. (S3) we arrive at Eq. (4).

*Time averages.* To obtain the time averaged MSD, we calculate the auxiliary integral

$$I(\tau) = \frac{1}{T-\tau}\int_0^{T-\tau}\langle x(t)x(t+\tau)\rangle dt. \quad \text{(S5)}$$

To this end, we use the representation of the hypergeometric function via the Fox $H$-function (see Eq. (1.131) in Ref. [2]) and then employ the integral over the $H$-function following Eq. (8.3.2.7) in Ref. [3], arriving at

$$I(\tau) = \frac{2^p p^{-2p}\Gamma(p+1)(D_0\tau)^{(p-1)/2}(D_0(T-\tau))^{(p+1)/2}}{\Gamma(p/2+1/2)\Gamma(1/2-p/2)} H^{3,1}_{3,3}\left[\frac{\tau}{T-\tau}\middle| \begin{array}{l}(1,1),\left(\frac{3}{2},1\right),\left(\frac{5}{2}+\frac{p}{2},1\right)\\ \left(\frac{3}{2}+\frac{p}{2},1\right),\left(\frac{1}{2}-\frac{p}{2},1\right),\left(1+\frac{p}{2},1\right)\end{array}\right]. \quad \text{(S6)}$$

Finally, we use Eq. (8.3.2.3) of Ref. [3] to get the result for the time averaged MSD (7).

*Approximative scheme for* EB. We now outline an approximative scheme to evaluate the ergodicity breaking parameter EB. Namely, from Eq. (S1) we express the particle displacement through $|x(t)| \sim |y(t)|^p$, where $y(t)$ is the Wiener process. Then, we take $\langle x^2(t)\rangle = (2D_0tp^{-2})^p$, which at $\Delta/T \ll 1$ yields $\left\langle\overline{\delta^2(\Delta)}\right\rangle \approx (2D_0p^{-2})^p\Delta/T^{1-p}$. Thus $\mathcal{EB}(\Delta) = \left\langle\overline{\delta^2(\Delta)}\right\rangle \Big/ \langle x^2(\Delta)\rangle \approx (\Delta/T)^{1-p}$, identical to the result in the main text derived from the exact approach (S1).

The fourth moment of the time averaged MSD in this approximative scheme becomes

$$\left\langle\left(\overline{\delta^2(\Delta)}\right)^2\right\rangle = \frac{1}{(T-\Delta)^2}\int_0^{T-\Delta}dt'\int_0^{T-\Delta}dt'' \times\langle[x(t'+\Delta)-x(t')]^2[x(t''+\Delta)-x(t'')]^2\rangle \quad \text{(S7)}$$

then becomes a combination of altogether 9 terms, each containing a product of four noise terms $\zeta(t)$. Using $\langle\zeta(t_1)\zeta(t_2)\zeta(t_3)\zeta(t_4)\rangle = \delta(t_1-t_2)\delta(t_3-t_4) + \delta(t_1-t_3)\delta(t_2-t_4) + \delta(t_1-t_4)\delta(t_2-t_3)$, the integrals from the Wiener processes disappear and two integrations are left.

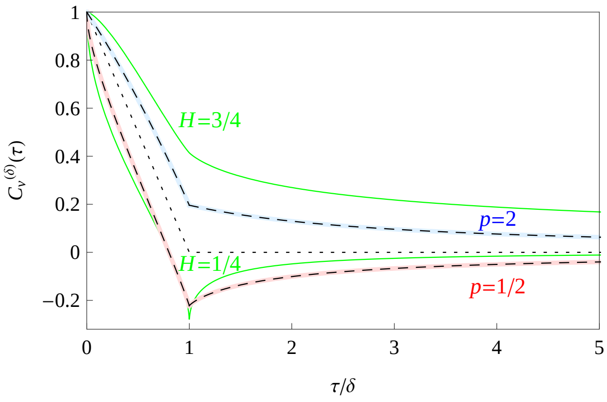


Figure S1: Normalized velocity autocorrelation function $C_v^{(\delta)}(\tau)$ for sub- and superdiffusion (dashed lines). The dotted curve corresponds to uncorrelated Brownian motion ($p = 1$), and the solid green curves represent fractional Brownian motion with the indicated Hurst coefficients (in the MSD, $p = 2H$).

These were evaluated numerically for a given value of $p$ to extract the scaling of the ergodicity breaking parameter

$$\mathrm{EB}(\Delta) = \frac{\left\langle \left(\overline{\delta^2}\right)^2 \right\rangle - \left\langle \overline{\delta^2} \right\rangle^2}{\left\langle \overline{\delta^2} \right\rangle^2} \tag{S8}$$

for $\Delta/T \ll 1$. Using the result $\langle \overline{\delta^2(\Delta)} \rangle^2 \propto \Delta^2$, we expand the fourth moment up to $\Delta^2$ to compute $\mathrm{EB}(\Delta/T \to 0)$, corresponding to the limit $T \to \infty$. For Brownian motion ($p = 1$) we find the correct scaling $\mathrm{EB} = (4/3)(\Delta/T)$. The scheme for HDPs with $p = 2$ yields $\mathrm{EB}(0) = 2/3$, close to the simulations results. Overall, this approximative scheme predicts that EB grows as the system deviates from the ergodic state $p = 1$ for both sub- and superdiffusion, see Fig. 5.

*Velocity autocorrelations.* We now determine the normalized velocity autocorrelation function

$$C_v^{(\delta)}(\tau) = \frac{\langle [x(\tau+\delta) - x(\tau)][x(\delta) - x(0)] \rangle}{\sqrt{\langle [x(\tau+\delta) - x(\tau)]^2} \sqrt{\langle [x(\delta) - x(0)]^2 \rangle}}. \tag{S9}$$

With the position autocorrelations (4), $C_v^{(\delta)}(\tau)$ becomes a universal function of $\delta/\tau$. $C_v^{(\delta)}(\tau)$ is plotted in Fig. S1. Thus, for superdiffusion the correlations remain positive, for subdiffusion $C_v^{(\delta)}(\tau)$ features a negative region mirroring the anti-persistence of the motion. In Fig. S1 we also show the complete decay of the correlations within the increment $\delta$ for Brownian motion. Moreover, we include the velocity autocorrelation function of fractional Brownian motion for the sub- and superdiffusive cases. The general behaviors are quite similar.

[1] H. Risken, The Fokker-Planck equation, (Springer-Verlag, Berlin, 1989).

[2] A. M. Mathai, R. K. Saxena, and H. J. Haubolt, The *H*-function (Springer, New-York, 2009).

[3] A. P. Prudnikov, Yu. A. Brychkov, and O. I. Marichev, Integrals and Series. Vol. 3: More Special Functions (Gordon & Breach Science Publishers, Amsterdam, 1998).
